# Supplementary material for: Intermittent "Turbulence" in a Many-body System
Source: arXiv:1901.10567 source file (2020-01-15)
Supplement: Supplementary file 1 [file supplemental.pdf]

# Supplemental Material — Intermittent "Turbulence" in a Many-body System

Guram Gogia, Wentao Yu, and Justin C. Burton
*Department of Physics, Emory University, Atlanta, GA, 30322*
(Dated: January 15, 2020)

**Supplementary Video 1**. Two cycles of melting and re-crystallization for a system consisting of 500 particles with $U_0 = 19$, $c_V$ =4% and $k_v = 800$ driven with $\phi = 18$. All quantities are given with units of $\lambda$, $m$, and $\sqrt{m/k_h}$ (length, mass, time). The left panel is the top view and the top right panel is the side view. The bottom right panel presents a graph for temporal evolution of $\Delta_{xy}$. Here is the link to the movie.

## I. NORMAL MODE ANALYSIS

The observed intermittent dynamics in our system arise from its inherent nonequilibrium and nonlinear nature. Nevertheless, an analysis of the harmonic vibrational modes in the system can shed light on how quenched disorder facilitates switching between states. We used dynamical matrix formalism to calculate the normal modes of the system [1–3]. The weighted Hessian matrix, $K$, was computed about the local potential energy minimum:

$$K_{ij} = \frac{\partial^2 V}{\partial r_i^\alpha \partial r_j^\beta}, \tag{1}$$

where $V$ is the total potential energy, including the external confining potentials, $i$ and $j$ denote the $i$th and $j$th particle, and $\alpha$ and $\beta$ denote $(x, y, z)$ coordinates. Using this harmonic approximation, Newton's 2nd law yields

$$M\ddot{\vec{x}} + K\vec{x} = 0, \tag{2}$$

where $\vec{\mathbf{x}}$ is the displacement vector of particle positions from equilibrium, and $M = \sqrt{m_i m_j}$. For $N$ particles in 3 dimensions, $M$ and $K$ are $3N \times 3N$ matrices and $x$ is the $3N \times 1$ vector. The dynamical matrix, $D = K/M$ has $3N$ eigenvalues which correspond to squares of the mode angular frequencies and the normalized eigenvectors represent the polarizations of the particle displacements.

In order to characterize the spatial extent of each mode, we calculated the participation ratio, $p_r$, for each eigenvector. $p_r$ characterizes the fraction of particles participating in a given vibrational mode:

$$p_r = \frac{(\sum_i |\hat{\mathbf{e}}_{m,i}|^2)^2}{N \sum_i |\hat{\mathbf{e}}_{m,i}|^4}, \tag{3}$$

where $\hat{\mathbf{e}}_{m,i}$ is the polarization vector of the $i$-th particle in the $m$-th unit eigenvector. The modes with $p_r$ close to unity represent coherent motion of a large fraction of particles, whereas the modes with $p_r \ll 1$ correspond to the localized motion of only a few particles.

## II. DERIVATION OF COUPLING BETWEEN VERTICAL AND HORIZONTAL MECHANICAL ENERGIES

In this system, particles are strongly confined in the vertical direction, and weakly confined in the horizontal directions, leading to a quasi-2D geometry. Energy is only delivered to the vertical direction due to white noise and is redistributed to the horizontal degrees of freedom due to nonlinearities. These nonlinearities occur when neighboring particles oscillate out-of-phase at high amplitude and their horizontal separation is small enough for them to scatter classically. We used the model of Rutherford scattering to estimate the rate of energy exchange between vertical and horizontal degrees of freedom during collisions.

Suppose two particles interact with a pairwise, repulsive, isotropic potential, $U(r)$. We consider elastic scattering with impact parameter $b$ and initial kinetic energy $E_0$ (Fig. S1). The linear momentum, angular momentum, and total mechanical energy are conserved. Let $v_r(t) = \frac{dr}{dt}$ and $v_\theta(t) = r\frac{d\theta}{dt}$ denote the radial and tangential velocity in the center-of-mass frame, respectively, and $m$ is the mass of each identical particle. Conservation of angular momentum and energy yields:

$$v_\theta(t) = \frac{J}{mr(t)} \tag{4}$$

$$v_r(t) = \sqrt{\frac{2}{m}\left(E_0 - U(r(t)) - \frac{mv_\theta(t)^2}{2}\right)}, \tag{5}$$

where $J = b\sqrt{2mE_0}$ is the angular momentum, and we have only considered the outgoing part of the scattering where $v_r > 0$. Dividing equation 4 by 5 yields

$$\frac{v_\theta(t)}{v_r(t)} = \frac{J}{r(t)\sqrt{2m(E_0 - U(r(t)) - \frac{mv_\theta(t)^2}{2})}}. \tag{6}$$

The left side of the equation also equals $\frac{1}{r}\frac{d\theta}{dt}\frac{dt}{dr}$. Cancelling out $dt$ and substituting for $v_\theta$ and $J$ results in:

$$\frac{d\theta}{dr} = \frac{b}{r\sqrt{r^2 - b^2 - r^2\frac{U(r)}{E_0}}}. \tag{7}$$

The particles come from infinitely far away prior to interacting. The closest distance to the center of mass that the particles can reach is $r_{min}$, which is the positive solution for

$$r^2 - b^2 - r^2\frac{U(r)}{E_0} = 0. \tag{8}$$

Assuming the incoming angle is $\theta(t = -\infty) = \pi$, then we add a negative sign since $J$ is negative, and at the closest approach ($r_{min}$), $\theta = \pi/2 + \theta_f/2$, where $\theta_f = \theta(t = \infty)$. Thus

$$\theta_f = \pi - 2\int_{r_{min}}^{\infty} \frac{b}{r\sqrt{r^2 - b^2 - r^2\frac{U(r)}{E_0}}}dr. \tag{9}$$

If we assume a Coulomb potential of the form $U = aE_0/r$, where $a$ is a characteristic interaction radius, then we may evaluate the integral, noting that the denominator is zero when $r = r_{min}$ (although the integral does not diverge):

$$\theta_f = \pi - 2\arctan\left(\frac{2b}{a}\right). \tag{10}$$

Ultimately we want the amount of kinetic energy transferred to perpendicular direction, which is:

$$E_0 \sin^2\theta_f = 16E_0\frac{a^2b^2}{(a^2 + 4b^2)^2}. \tag{11}$$

Here we have assumed a long-ranged Coulomb potential. However, our simulations use a finite-ranged, screened potential. In the case of hard spheres of radius $R$, the scattering formula is nearly the same as in Eq. 11, except that $a$ is replaced with $4R$.

### A. Case 1: Energy is mostly in horizontal degrees of freedom

The potential energies associated with the external confinement of particles are independent, i.e. the depend only on $r$ or $z$. As a result, mechanical energy can be divided into vertical and horizontal energy. In each direction, kinetic and potential energy is assumed to be equipartitioned. Since the particles strongly confined in $z$, collisions are mostly determined by kinetics within the $xy$-plane. The frequency of collision between particles, $f_c$, is:

$$f_c = v_h a\rho, \tag{12}$$

where $\rho$ is the surface density of the particles, $a$ is the typical spacing, and $v_h$ is the average horizontal velocity. As the energy is mainly in the horizontal direction, the vertical energy $E_v$ can be expressed as

$$E_v = k_v\delta b^2 = mv_v^2, \tag{13}$$

where $k_v$ is the strength of vertical confinement, $v_v$ is the average vertical velocity, $m$ is the particle mass, and $\delta b$ is average vertical displacement from equilibrium position. Since particles can have different masses, on average there

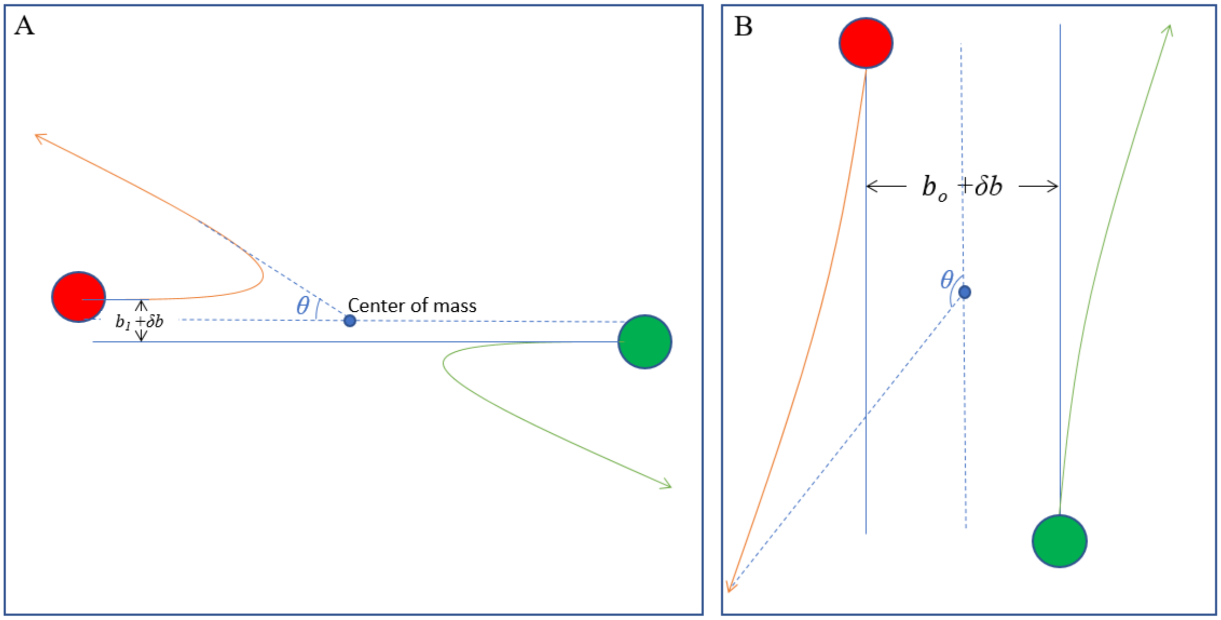


Figure S1. A sketch of the two scattering processes considered for energy transfer, both in the center-of-mass frame. The two limiting cases correspond to when all the energy is in the (A) horizontal direction or the (B) vertical direction.

is a gap between the vertical equilibrium position of each particle, denoted as $b_1$, which is dependent on $c_v$. $b_1 + \delta b$ gives the impact parameter of one collision (see Fig. S1A). After each collision, a portion of kinetic energy $\Delta E$ is transferred from the horizontal to the vertical direction:

$$\Delta E_v(\delta b) = \frac{E_h \sin^2 \theta_f}{2} \approx \frac{8a^2 E_h (b_1 + \delta b)^2}{\left(a^2 + 4(b_1 + \delta b)^2\right)^2}. \tag{14}$$

We are only interested in the amount of energy transferred due to the excess vertical displacements, $\delta b$. Therefore, the net energy transferred is:

$$|\Delta E_v(\delta b) - \Delta E_v(0)| \approx \frac{16a^2 b_1 E_h \left(a^2 - 4b_1^2\right)}{\left(a^2 + 4b_1^2\right)^3}\delta b. \tag{15}$$

The total rate of energy transfer from the horizontal to vertical direction, $p_{h\to v}$, is proportional to the above quantity multiplied by the collision frequency (Eq. 12). Since $v_h \propto E_h^{1/2}$ and $\delta b \propto E_v^{1/2}$ (Eq. 13), the power of energy transfer is

$$p_{h\to v} \propto E_h^{\frac{3}{2}} E_v^{\frac{1}{2}}. \tag{16}$$

### B. Case 2: Energy is mostly in vertical degrees of freedom

This case is more important for the recurrent energy cascades since the energy is constantly driven into the vertical direction, leading to vertical oscillations, with subsequent scattering events that transfer energy to the horizontal direction. Figure S1B illustrates this case. The derivation here is identical to Case 1, except the role of vertical and horizontal energies are reversed. However, the collision rate is still dependent on the horizontal energy since the particles are strongly confined in $z$.

Thus, we have:

$$p_{v\to h} \propto v_h v_v^2 \delta b \propto E_h E_v \tag{17}$$

since $\delta b \propto E_h^{1/2}$. Thus the fundamental asymmetry in the two cases comes from the fact that the collision rate only depends on the average horizontal velocities.

### C. Application to minimal model

For simplicity, we combine these two terms and assume that both types of scattering events can occur simultaneously, this model gives the result that the net power of energy transferred from vertical to horizontal is:

$$p_{v\rightarrow h,net} \approx c_1(E_v E_h)(1 - c_2\sqrt{\frac{E_h}{E_v}}), \tag{18}$$

where $c_1$, $c_2$ are constants independent of energy. In our minimal model, we assume that $c_1 = c$ and $c_2 = 1$ for simplicity. Consequently, if $E_v = E_h$, no net energy is transferred between the degrees of freedom.

As mentioned, both in experiment and simulation, Case 2 is the most common, and Case 1 is only important in the gas-like state. In fact, the quantity $b_1$ is very small or zero in most cases, i.e. if there is no vertical energy, the particles rest in the same plane. Nevertheless, we have kept terms linear in $\delta b$ for simplicity and symmetry. Although this is only a rudimentary model, assuming Coulomb interaction, it captures the appropriate scaling of $E_v$ and $E_h$, and is based on physical processes and kinetics in the experiment and particle simulation.

## III. CALCULATION OF THE EXCITED AND QUIESCENT LIFETIMES

The excited and quiescent states in the minimal model are separated using a threshold algorithm. Throughout an entire time series, we define the excited state as times when $A/\langle B\rangle > 0.02$, where $\langle B\rangle$ represents the average over the entire time series. After the initial thresholding, some excited (quiescent) periods are very short. Quiescent periods that are shorter than 3 time units are identified and removed while the two neighboring excited periods are concatenated. The remaining short excited periods which are less than 3 time unites are not counted in the distributions. An example of distributions for quiescent and excited periods with $\Theta = 48$ are presented in Fig. S9. The entire time series is $10^6$ time units.

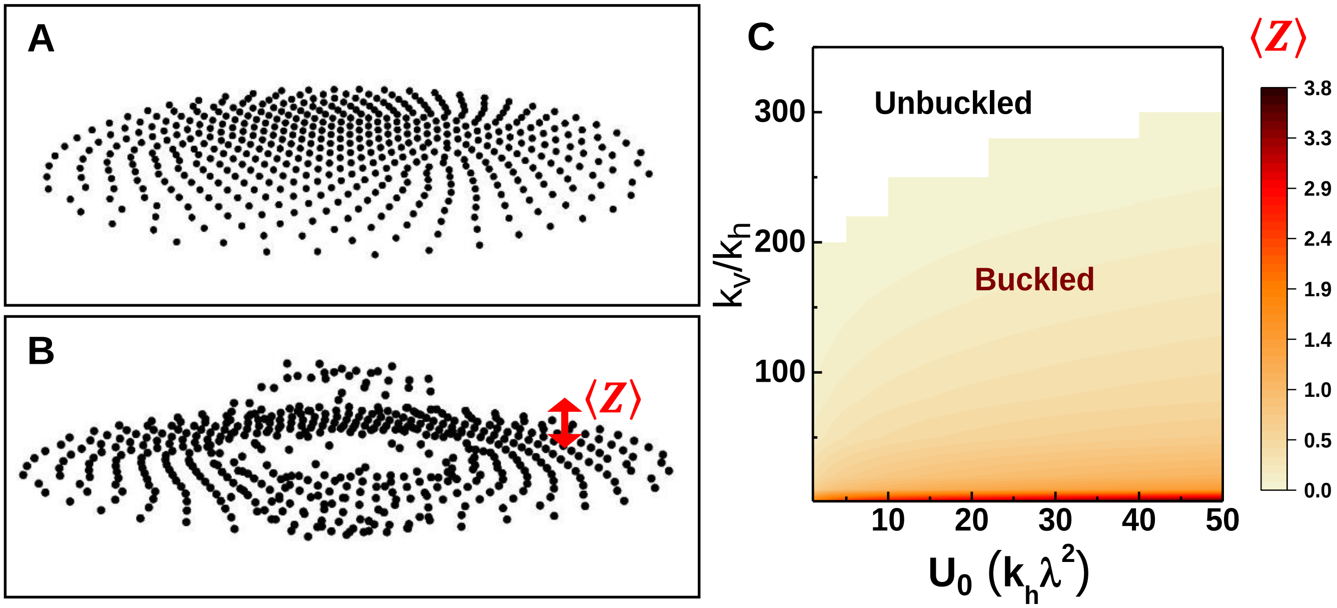


Figure S2. (A) Unbuckled layer of particles for $U_0/k_h\lambda^2 = 19$ and $k_v/k_h = 800$. Decreasing the value of $k_v/k_h$ to 200 results into a buckled phase (B), which is characterized by the standard deviation of particle positions in the $z$-direction, $\langle Z\rangle$. (C) Color map showing $\langle Z\rangle$ as a function of $U_0/k_h\lambda^2$ and $k_v/k_h$.

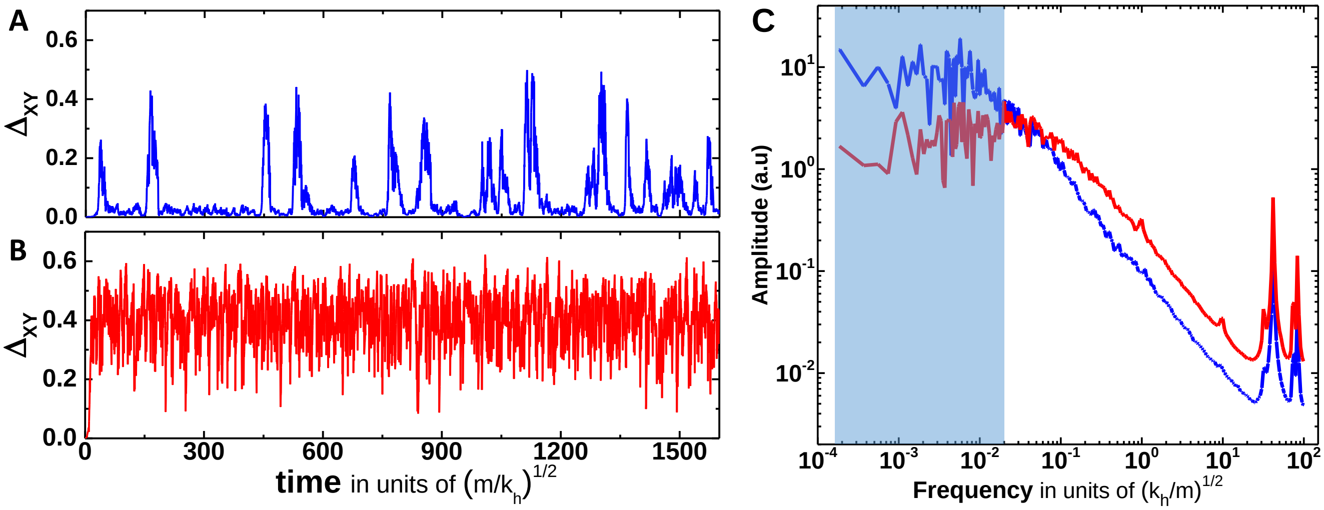


Figure S3. Intermittent dynamics for polydisperse systems. (A) Fractional kinetic energy, $\Delta_{xy}$ for a system of 500 particles with $c_V = 5\%$ and $\phi = 12$. Increasing $\phi$ to 30 results into a perpetually melted state (B). The parameters in the simulations were: $\gamma = 0.2$, $U_0 = 19$, and $k_v = 800$. (C) Amplitude of Fourier transforms for data shown in panels A (blue) and B (red). The blue box represents the area of integration of the Fourier transform below $\omega = 0.02$.

---

[1] S. Henkes, C. Brito, and O. Dauchot, Extracting vibrational modes from fluctuations: a pedagogical discussion, Soft Matter **8**, 6092 (2012).

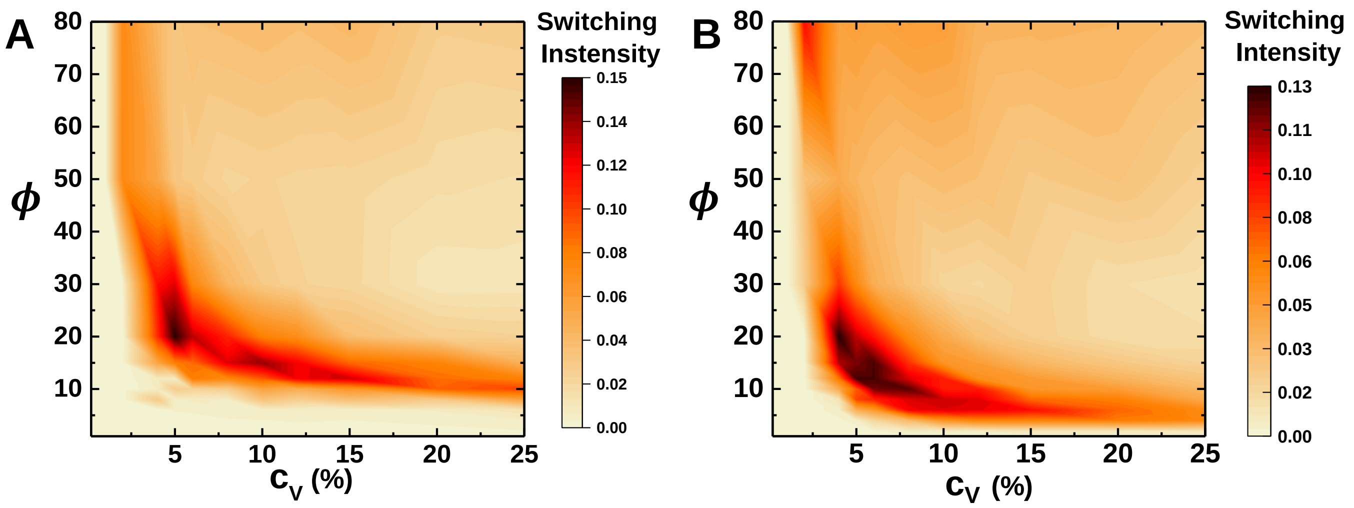


Figure S4. Heatmaps of switching intensity for a system comprised of 500 particles for (A) $k_v = 1000$ and (B) $k_v = 600$. The following parameters were used in the simulations: $U_0 = 19$ and $\gamma = 0.2$.

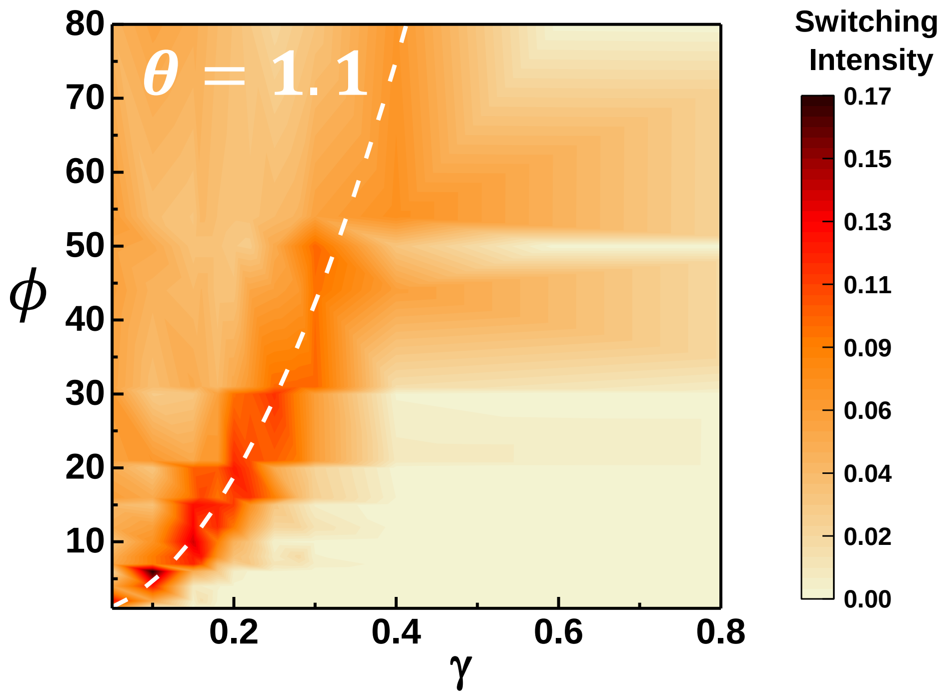


Figure S5. Heatmap of switching intensity for a system comprised of 500 particles with $U_0 = 19$, $c_v = 6\%$, and $k_v = 800$ as a function of $\phi$ and $\gamma$.

[2] A. Bottinelli and J. L. Silverberg, How to: Using mode analysis to quantify, analyze, and interpret the mechanisms of high-density collective motion, Front. Appl. Math. Stat. **3**, 26 (2017).
[3] J. Burton and S. Nagel, Echoes from anharmonic normal modes in model glasses, Phys. Rev. E **93**, 032905 (2016).

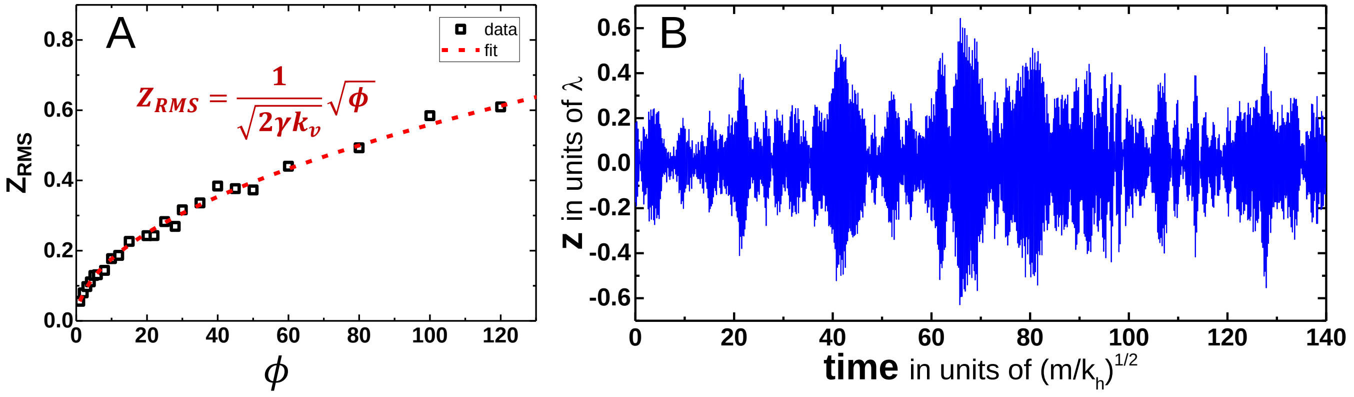


Figure S6. (A) Root Mean Square (RMS) of the oscillation amplitude in $z$ of a single particle as a function of $\phi$, $\gamma = 0.2$ and $k_v = 800$. The dashed red line is the analytic prediction for a damped, stochastically-driven harmonic oscillator. (B) $z$-position of a single particle in a sample of 500 particles that is forced at $\phi = 18$. The system melts at time $= 70$ due to the large preceding oscillation amplitude.

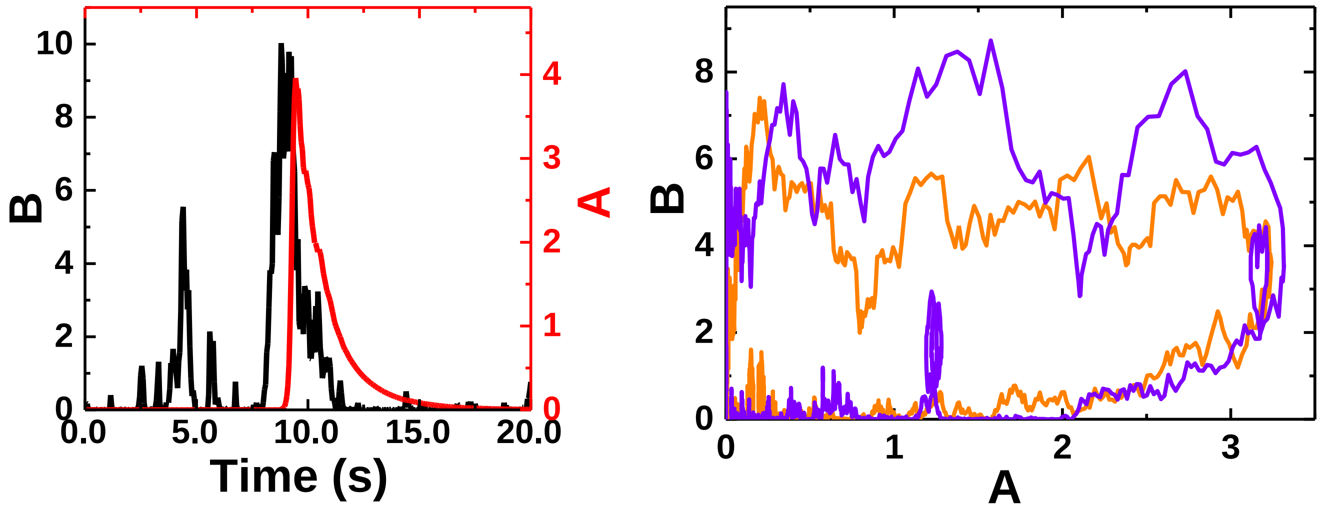


Figure S7. (Left) Temporal evolution of A and B over 20 units in time with $c = 1.5$, $\Phi = 10$, and $\gamma = 0.5$. (Right) Phase portrait of two separate cascades in energy for the same parameters.

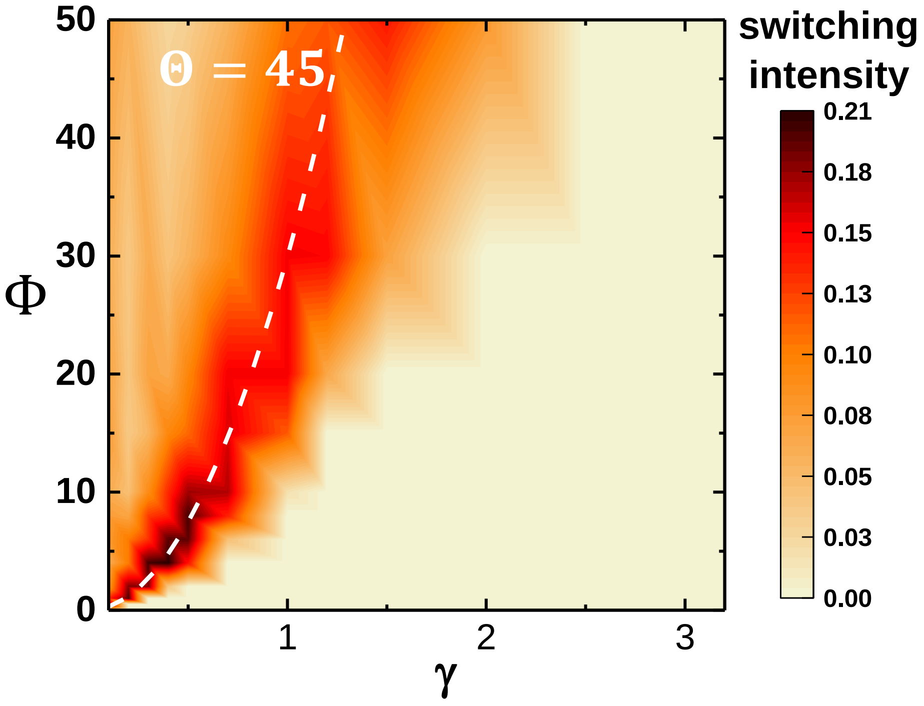


Figure S8. Heatmap of switching intensity of $R \equiv A/(A+B)$ for a range of $\Phi$ and $\gamma$ with $c = 1.5$. As a reminder, $\Theta = c\Phi/\gamma^2$

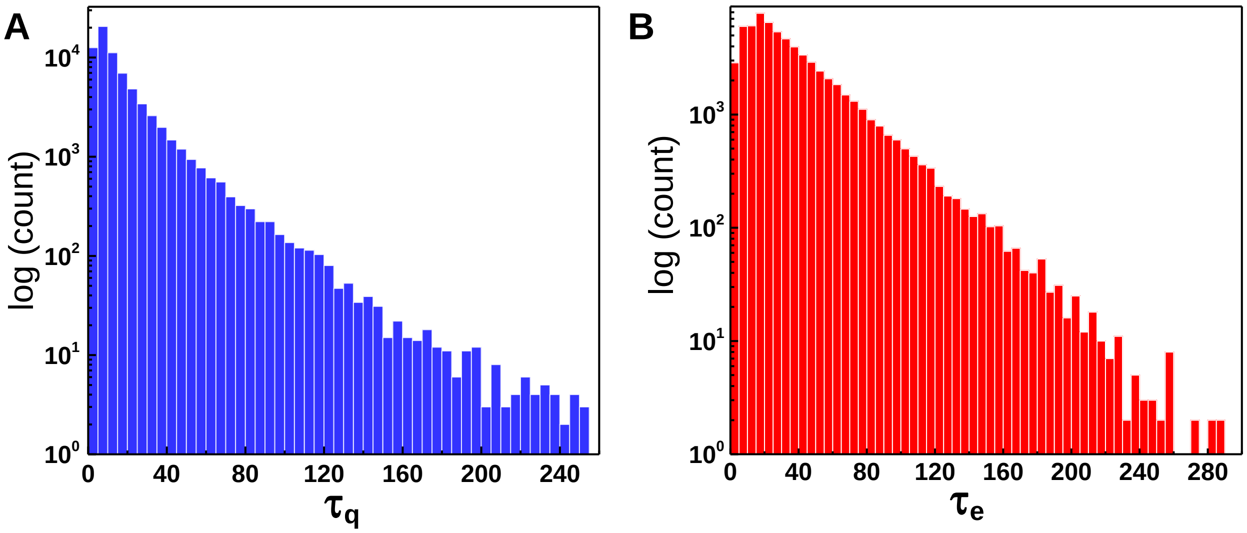


Figure S9. Distributions of durations of quiescent ($\tau_q$) and excited ($\tau_e$) states for $\Theta = 48$. Both $\tau_q$ and $\tau_e$ have exponential tails at large $\tau$, which is especially true for $\tau_e$.
